# Supplementary material for: Nonlinear Dynamics in the Formation of Molecular Polariton Condensates
Source: arXiv:2505.08674 source file (2025-05-13)
Supplement: Supplementary file 1 [file SI.pdf]

# Supplementary Information: Nonlinear Dynamics in the Formation of Molecular Polariton Condensates

(Dated: May 13, 2025)

## I. EXPERIMENTAL METHODS

### Sample Preparation:

The $SiO_2/TiO_2$ DBR substrates were first treated with oxygen plasma for approximately 5 minutes to promote better spreading of the R3B-SMILES PMMA solution. The synthesis of the R3B-SMILES complex is described in [1]. The solution was then deposited using a three-step spin-coating process. Approximately 70 $\mu$L of the solution was dispensed onto each plasma-treated substrate. Spin-coating was performed in two stages: 2000 rpm for 15 seconds followed by 4000 rpm for 120 seconds. The resulting films were dried in the dark at room temperature under vacuum ($\sim$ 2500 Pa) for 48 hours to ensure uniform solvent evaporation. Film thickness was assessed using a Bruker Dektak-XT profilometer and found to be approximately 35 nm, consistent over a lateral area of 1500–2000 $\mu m^2$. For the higher-Q cavity which forms a condensate, a 100 nm silver top mirror was then deposited by electron-beam evaporation at a rate of 0.2 Å/s to complete the optical cavity structure. The lower-Q cavities have a 30 nm silver top mirror to allow for sufficient transmission or reflection.

### ECPL spectroscopy:

The pump pulses at 515 nm are the second harmonic of a pulsed femtosecond laser (Light Conversion, Pharos PH1-20-0200-02-12) operating at 1 kHz with a pulse duration of $\sim$200 fs. The beam is separated by a 50/50 plate beamsplitter (EKSMA) centered at 515 nm. One beam is sent into a motorized delay stage (Thorlabs, LTS300) to vary the delay between the two pulses, while each beam is individually frequency modulated by a chopper wheel at frequencies 285 Hz and 203 Hz. The two beams are recombined in a parallel geometry and focused onto the sample with a microscope objective (20X Mitutoyo Plan Apo Infinity Corrected Long WD). Due to the fact the sample is subject to degradation under prolonged laser excitation, it is placed on a linear stage that oscillates continuously between two points spaced approximately 1 mm apart from each other. The photoluminescence is collected in reflection and directed towards a photodetector with a dichroic mirror with a cut-on wavelength at 550 nm (Thorlabs, DMSP550). A notch filter at 515 nm is placed in front of the photodetector to ensure that the pump has been completely filtered out. To extract the nonlinear contribution to the photoluminescence signal (ECPL), the photode-

tector is connected to a lock-in amplifier (Zurich Instruments, HF2LI), where the signal is demodulated at the sum-frequency of the two pulses (488 Hz). Four scans of the dynamics are recorded for each fluence and averaged together. As the oscillations from the sample movement introduce periodic oscillations in the signal due to sample inhomogeneity and varying distance from the objective to the sample, the "true" ECPL signal is obtained by removing these oscillations via Fourier filtering (see section III).

**$k$-space resolved photoluminescence:**

Measurements were performed using a custom-built optical setup designed for momentum-space imaging. Excitation was provided by a laser source coupled into a Princeton Instruments monochromator (514 nm), and the emitted PL was detected using a PIXIS: 256 electron-multiplying charge-coupled device (EMCCD) camera. A high numerical aperture (NA = 0.8), 50× objective lens was employed to collect the emission. To enable momentum-resolved detection, the back focal plane of the objective was imaged directly onto the EMCCD camera. This configuration allowed single-shot acquisition of angular dispersion of the emitted photons.

## II. SIMULATION AND PARAMETER DETAILS

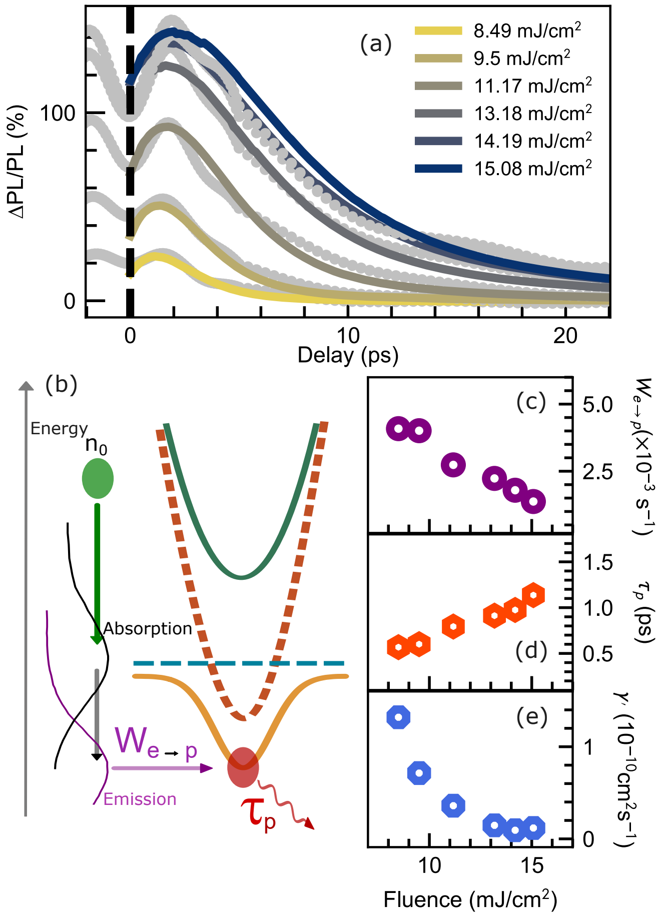


Fig. S1. (a) The experimental ECPL dynamics are reproduced in gray for a range of fluences above the condensation threshold. The fitted simulations from the semi-classical Boltzmann equations are plotted over the data (blue-yellow). (b) Energetic structure of the R3B-SMILES system. The non-resonant excitation creates a population, $n_0$, that thermalizes quickly to the dark state reservoir. The reservoir radiatively pumps and populates the LP branch ($W^{e \to p}$). The emission from the LP happens on a timescale that is related to the polariton lifetime, $\tau_p$. (c)-(e) Plots of the density dependence on various fit parameters in our model. Each plot shows that the rates were forced to decrease in order to fit the dynamics.

### Hopfield coefficients:

Modeling of the Jaynes-Cummings model using the QuTip package in python allows us to compute and reproduce the polariton dispersion from [1], as well as the Hopfield coefficients, shown in Fig. S2 below:

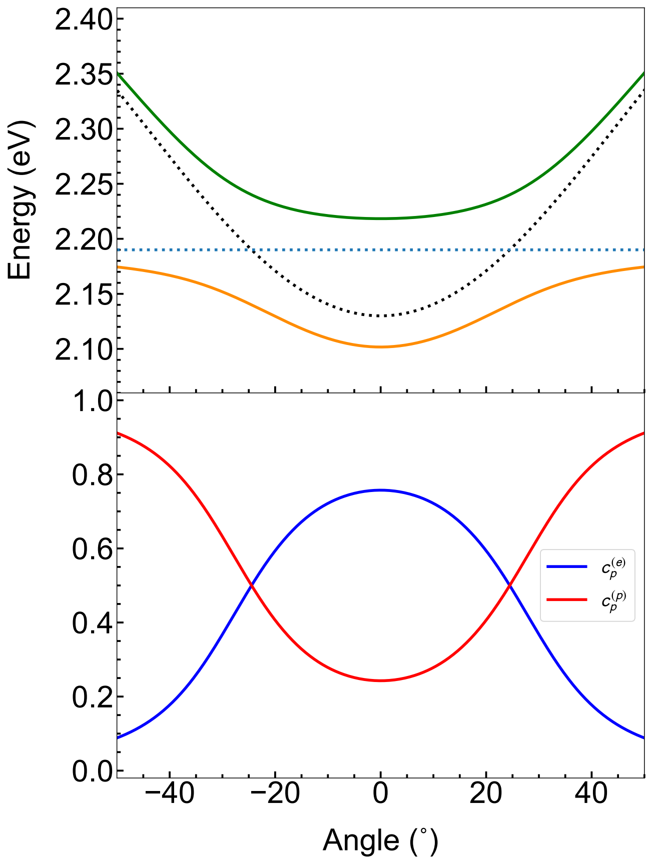


Fig. S2. (a): Dispersion relationship showing the upper (green) and lower (orange) polariton branches. The exciton dispersion (dotted, blue) and the cavity dispersion (dotted, black) are also shown. (b) Hopfield coefficients for the lower polariton branch.

## Exciton lifetime

To estimate the exicton lifetime, the ECPL dynamics of R3B-SMILES bare film at 1.27 $mJ/cm^2$ are fit to the form of [2]:

$$I_{NPL} \approx \ln\left(1 - \frac{\alpha^2 \exp\left(-\Gamma_e \tau\right)}{1+\alpha^2}\right), \alpha = \frac{n_0 \Gamma_e}{\gamma'} \tag{1}$$

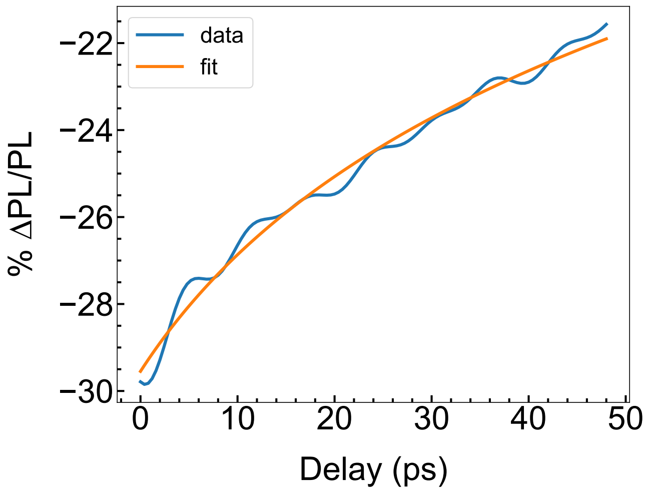


Fig. S3. Fit of Bare Film ECPL @ 1.27 mJ/cm$^2$

Both $\Gamma_e$ and $\gamma'$ are free parameters in the fit, where $\Gamma_e$, is monomolecular decay rate of the exciton, and $\gamma'$ is the bimolecular quenching rate. From $\Gamma_e$, we can determine $\tau_e = \frac{1}{\Gamma_e}$.

**Initial excitation density:**

The absorbed photon density is given by [3]:

$$n_0 = \frac{\overline{P}\lambda}{R \times c \times h \times \pi \times (\frac{D}{2})^2 \times \delta}, \tag{2}$$

where $\overline{P}$ is average power, $\lambda$ is the excitation wavelength (515 nm), R is the repetition rate of the laser (1 kHz), D is the spot diameter ($\approx$ 5 $\mu$m, estimated), and $\delta$ is the penetration depth (35 nm, thickness of film).

## III. DATA TREATMENT

As the the sample was continuously oscillating during the measurement due to degradation, a low frequency noise persisted throughout our data sets, as shown in the raw ECPL plot in Fig. S4:

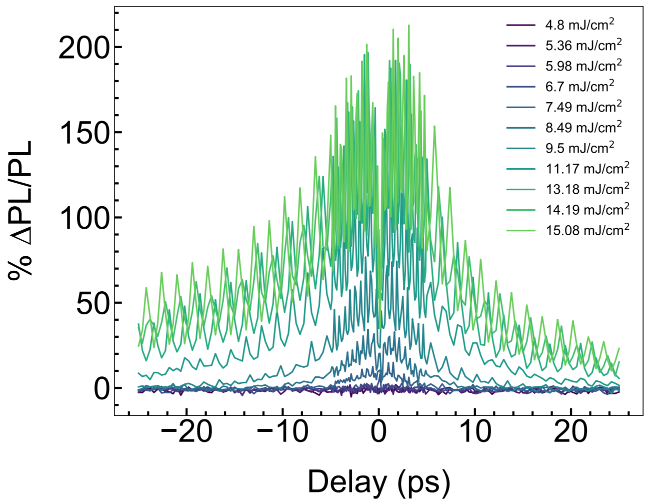


Fig. S4. Raw ECPL dynamics

To remove the contributions from the oscillations, we first compute and plot the Fourier transform of the raw signal, shown in Fig. S5:

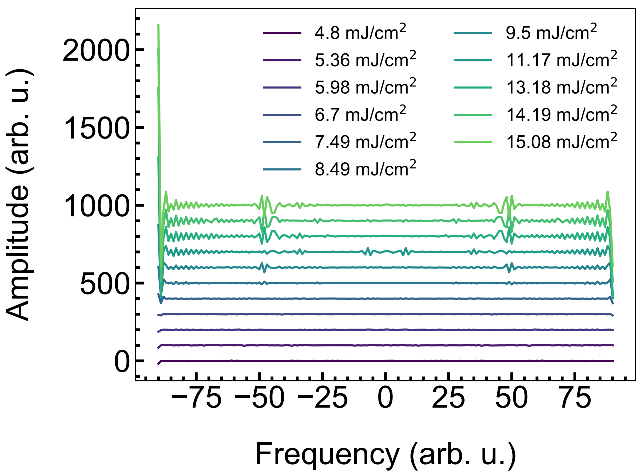


Fig. S5. Fourier Transform of Raw ECPL data. Plots are offset for clarity.

The low frequency components are set to 0, as shown in Fig. S6. After performing the inverse Fourier transform, the oscillations are removed as in Figure 2 in the main text.

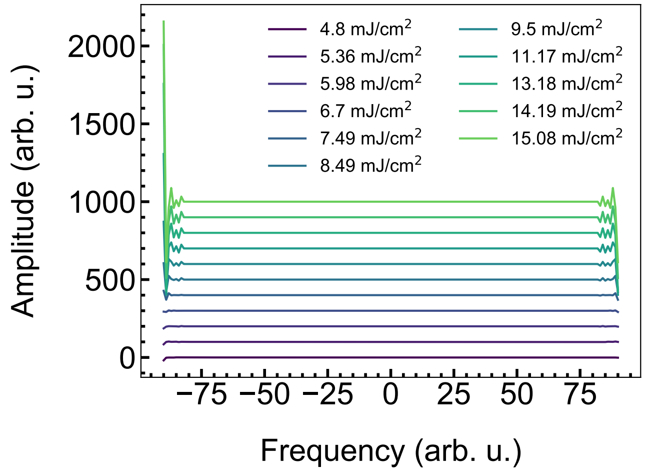


Fig. S6. Fourier Transform of ECPL data with low-frequency noise reduced. Plots are offset for clarity.

## IV. ECPL DYNAMICS OF LOWER-Q CAVITY

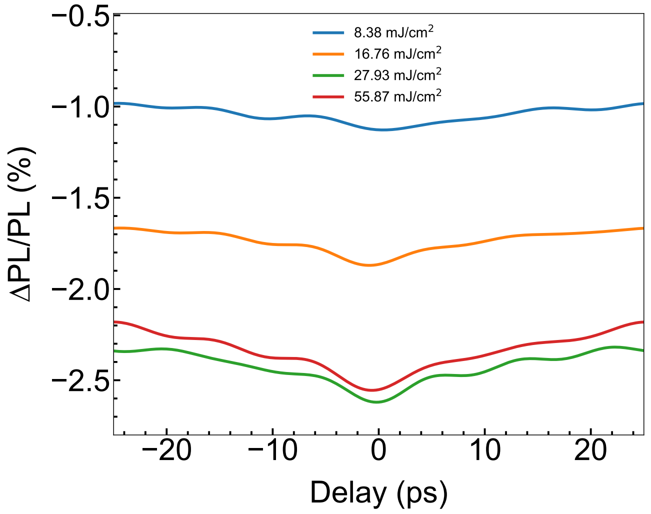


Fig. S7. ECPL dynamics of lower-Q cavity

The reservoir dynamics of the lower-Q cavity are shown in S7, which does not form a condensate, is dominated by a negative nonlinear signal due to bimolecular annihilation processes.

## V. TRANSIENT REFLECTION MEASUREMENTS

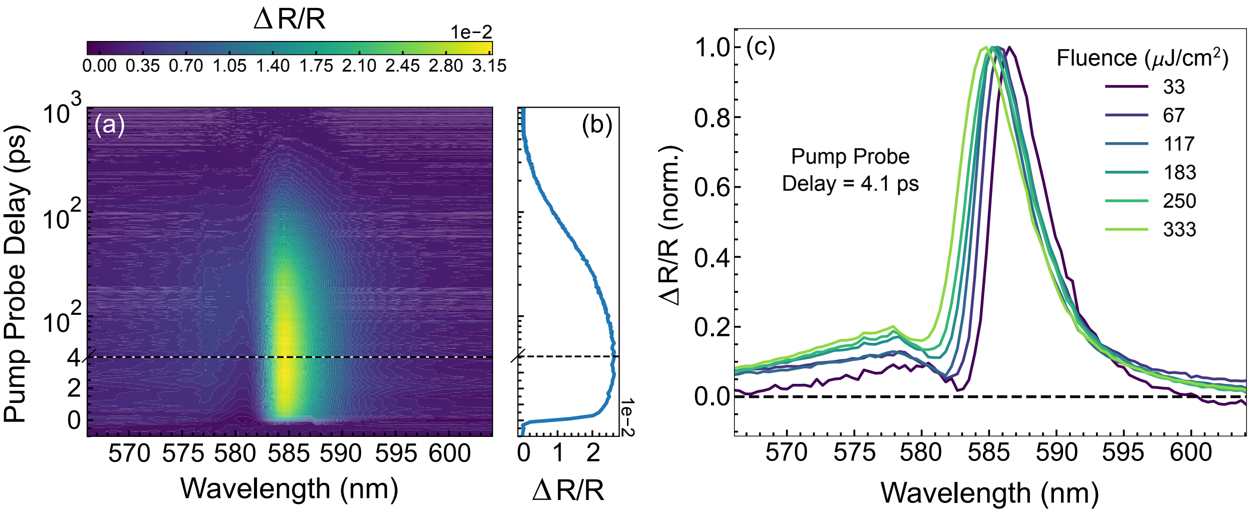


Fig. S8. (a) Transient reflection map of Lower-Q cavity at fluence of 737 $\mu$J/cm$^2$. (b) Time-delay cut of transient reflection map at peak intensity. (c) Intensity dependence of cuts along the wavelength axis of the transient reflection maps at a delay of 4.1 ps, indicated increased population at higher-lying $k$-states.

Figure S8(a) presents transient reflectance spectra as a function of pump-probe delay, acquired using a non-resonant excitation at 515 nm, mirroring the conditions of our ECPL measurements. Our experimental scheme selectively probes the $\vec{k} = 0$ point in the polariton dispersion (see Methods). A prominent spectral feature emerges at around 600-610 nm, corresponding to the population in the lower polariton state. This feature's spectral intensity reaches its peak within a few picoseconds, indicating a relatively slow transfer of photo-excited population into the lower polariton state. We anticipate that the peak intensity would be reached more rapidly in cavities with higher quality factors and longer polariton lifetimes, such as those utilized for ECPL measurements. This observation thus supports our assertion that the radiative pumping rate in R3B-SMILES cavities occurs on the order of hundreds of femtoseconds. However, this analysis alone does not reveal the presence of any additional sources of population for the $\vec{k} = 0$ state.

The experimental geometry of our transient reflection measurement allows us to observe changes in the population across a small range of higher energy k-states around $\vec{k} = 0$ under different experimental conditions. After a non-resonant excitation of the system, the

population in the dark state reservoir radiatively pumps the lower polariton at $\vec{k} = 0$, as well as higher lying k-states due to the broadband photoluminescence spectrum of the bare R3B-SMILES film. Under increased pump fluence, as seen in Fig. S8(c), we see that the population in the higher-lying k-states begins dominating the bleach signal, as evidenced by the blue-shifting of the peak. Parametric scattering of polaritons throughout the lower polariton dispersion, especially at $\vec{k} = 0$, can explain the shift in the population [4]. If we are not saturating the density of states, the population at higher k-points can be explained by parametric scattering of lower polaritons at lower-energy k-points. Despite the Frenkel-like excitations seen in organic materials, evidence of polarition pair-scattering has been reported in [1], where a blueshifting of the spectrum can be seen above the condensation threshold [4]. Polariton-polariton scattering has also been reported across various other organic systems [5–7].

## VI. REFERENCES


[1] P. Deshmukh, S. Satapathy, E. Michail, A. H. Olsson, R. Bushati, R. K. Yadav, M. Khatoniar, J. Chen, G. John, B. W. Laursen, *et al.*, Plug-and-play molecular approach for room temperature polariton condensation, ACS Photonics **11**, 348 (2024).

[2] E. Rojas-Gatjens, K. M. Yallum, Y. Shi, Y. Zheng, T. Bills, C. A. Perini, J.-P. Correa-Baena, D. S. Ginger, N. Banerji, and C. Silva-Acuña, Resolving nonlinear recombination dynamics in semiconductors via ultrafast excitation correlation spectroscopy: Photoluminescence versus photocurrent detection, The Journal of Physical Chemistry C **127**, 15969 (2023).

[3] L. Mazza, S. Kéna-Cohen, P. Michetti, and G. C. La Rocca, Microscopic theory of polariton lasing via vibronically assisted scattering, Physical Review B—Condensed Matter and Materials Physics **88**, 075321 (2013).

[4] T. Yagafarov, D. Sannikov, A. Zasedatelev, K. Georgiou, A. Baranikov, O. Kyriienko, I. Shelykh, L. Gai, Z. Shen, D. Lidzey, *et al.*, Mechanisms of blueshifts in organic polariton condensates, Communications Physics **3**, 18 (2020).

[5] K. Daskalakis, S. Maier, R. Murray, and S. Kéna-Cohen, Nonlinear interactions in an organic polariton condensate, Nature materials **13**, 271 (2014).

[6] J. Kasprzak, M. Richard, S. Kundermann, A. Baas, P. Jeambrun, J. M. J. Keeling, F. Marchetti, M. Szymańska, R. André, J. Staehli, *et al.*, Bose–einstein condensation of exciton polaritons, Nature **443**, 409 (2006).

[7] G. Lerario, D. Ballarini, A. Fieramosca, A. Cannavale, A. Genco, F. Mangione, S. Gambino, L. Dominici, M. De Giorgi, G. Gigli, *et al.*, High-speed flow of interacting organic polaritons, Light: Science & Applications **6**, e16212 (2017).
